# Supplementary material for: Ultrafast ab-initio Quantum Chemistry Using Matrix Product States
Source: arXiv:1902.08489 source file (2019-02-22)
Supplement: Supplementary file 1 [file supporting_info.pdf]

# Supporting Information: Ultrafast ab-inito Quantum Chemistry Using Matrix Product States

Lars-Hendrik Frahm* and Daniela Pfannkuche

*I. Institut für Theoretische Physik, Universität Hamburg, Jungiusstraße 9, 20355 Hamburg, Germany*

E-mail: lfrahm@physnet.uni-hamburg.de

# 1 Convergence of the time step size for propagation of the hydrogen chain

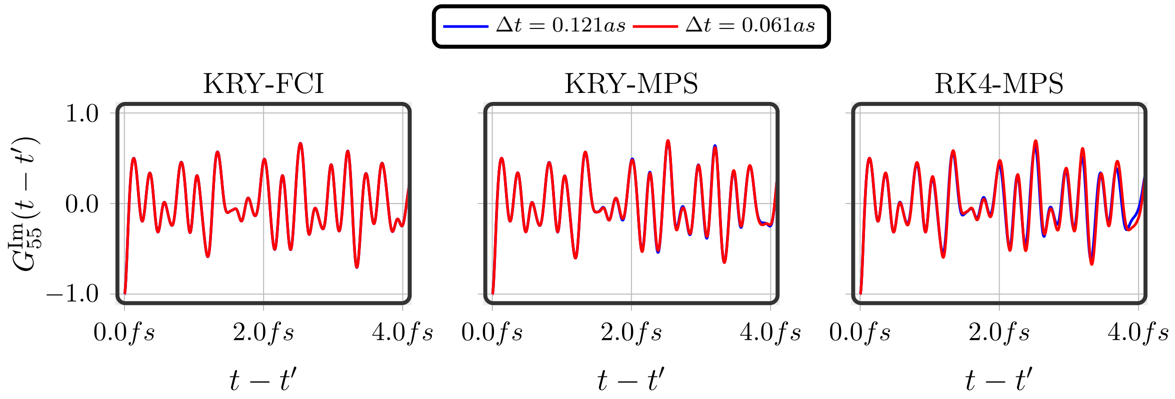


Figure 1: (left) The imaginary part of the one-particle Green's function calculated using the quasi exact full CI approach for the many-electron state representation and the Krylov time evolution method to solve the time-dependent Schrödinger equation. The Krylov space is spanned from five $N_K = 5$ orthonormal basis vectors and the time step size is $\Delta t = 0.121as$ (blue) and $\Delta t = 0.061as$ (red). (middle) The imaginary part of the one-particle Green's function calculated using the MPS approach for the many-electron state representation and the Krylov time evolution method to solve the time-dependent Schrödinger equation. The Krylov space is spanned from five $N_K = 5$ orthonormal basis vectors and the time step size is $\Delta t = 0.121as$ (blue) and $\Delta t = 0.061as$ (red). (right) The imaginary part of the one-particle Green's function calculated using the MPS approach for the many-electron state representation and the fourth-order Runge-Kutta method to solve the time-dependent Schrödinger equation. The the time step size is $\Delta t = 0.121as$ (blue) and $\Delta t = 0.061as$ (red).

# 2 Convergence of the time step size for propagation of the hydrogen chain

## References

(1) Kraus, P. M.; Mignolet, B.; Baykusheva, D.; Rupenyan, A.; Horný, L.; Penka, E. F.; Grassi, G.; Tolstikhin, O. I.; Schneider, J.; Jensen, F.; Madsen, L. B.; Bandrauk, A. D.; Remacle, F.; Wörner, H. J. Measurement and laser control of attosecond charge migration in ionized iodoacetylene. *Science* **2015**, *350*, 790–795.

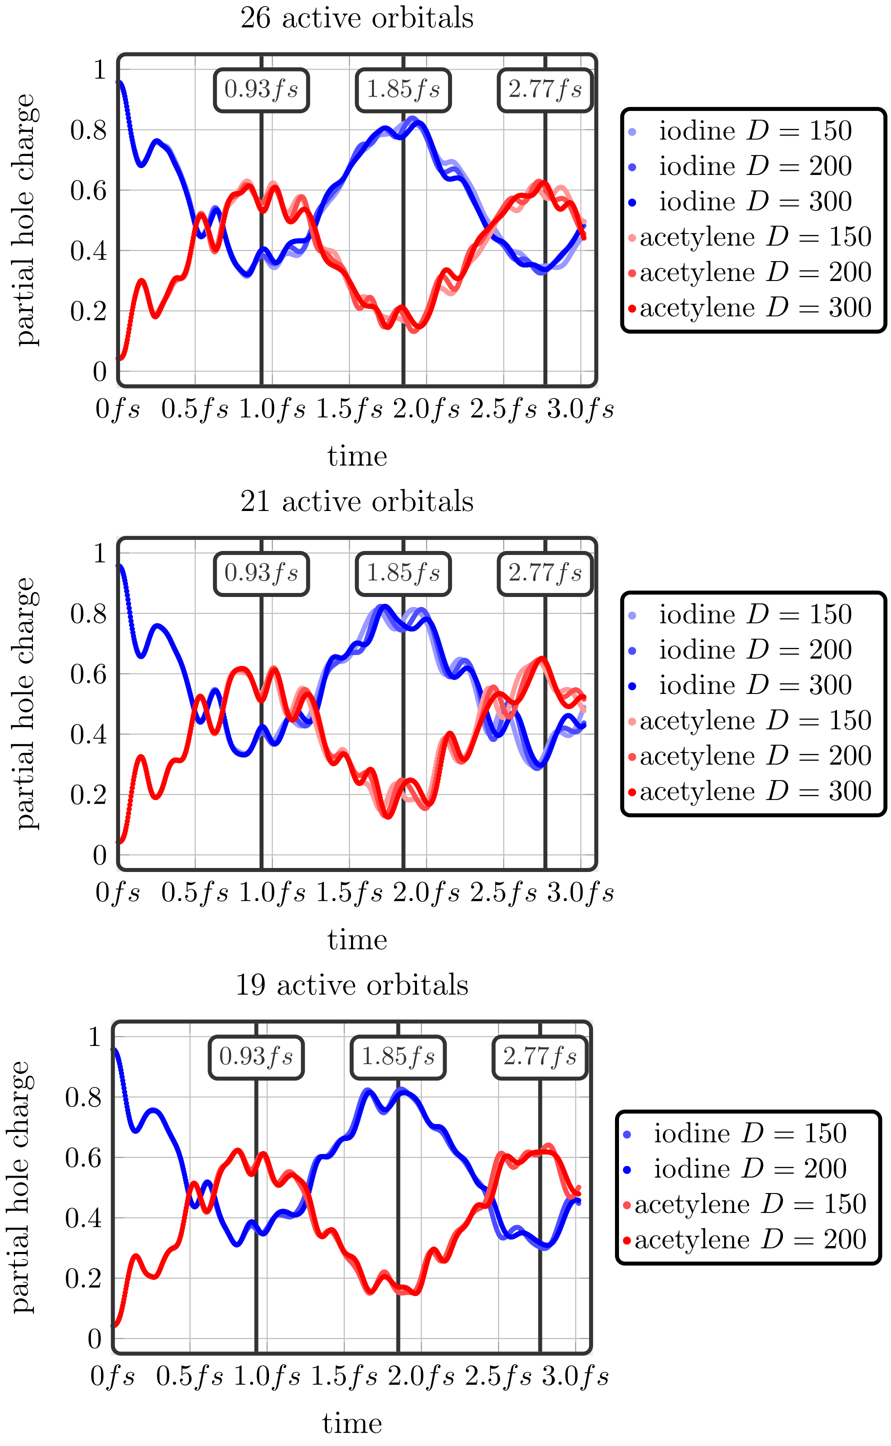


Figure 2: Convergence of the partial trace with the number of active orbitals and the MPS bond dimension for the ionized iodoacetylene molecule. The Krylov space dimension is $N_K = 5$ for all calculations and the time step size is $1as$. Special points from the experiment by Kraus et al.[1] are highlighted for reference.
